# Supplementary material for: Symmetrization of Localized Molecular Orbitals
Source: arXiv:2302.13654 ancillary file (2023-04-25)
Supplement: Supplementary file 1 [file si.pdf]

# Supporting Information: Symmetrization of Localized Molecular Orbitals


Jonas Greiner† and Janus J. Eriksen*,‡

†*Department Chemie, Johannes Gutenberg-Universität Mainz*

*Duesbergweg 10–14, 55128 Mainz, Germany*

‡*DTU Chemistry, Technical University of Denmark*

*Kemitorvet Bldg. 206, 2800 Kgs. Lyngby, Denmark*

E-mail: janus@kemi.dtu.dk


## Gradient and Hessian of objective function

The gradient, the diagonal of the Hessian, and the Hessian multiplied by some trial function are given by the contributions to specific blocks of these matrices depending on whether the considered elements are inside or outside of $S_1$ and $S_2$.

### Elements added to gradient $\frac{d\mathcal{J}}{d\kappa_{rs}}$

$r \in S_1$:

$$-2\sum_{G}^{h}\sum_{(S_1,S_2)\in\mathcal{S}_G}\sum_{\bar{q}\notin S_2}\sum_{\mu\nu\sigma\rho} c'^{*}_{\mu r}c^{*}_{\sigma s}c'_{\nu\bar{q}}c'_{\rho\bar{q}}G_{\mu\nu}G_{\sigma\rho} \tag{1}$$

$s \in S_1$: Negative transpose of $r \in S_1$

$r \notin S_2$:

$$-2\sum_{G}^{h}\sum_{(S_1,S_2)\in\mathcal{S}_G}\sum_{p\in S_1}\sum_{\mu\nu\sigma\rho} c'_{\nu r}c_{\rho s}c'^{*}_{\mu p}c'^{*}_{\sigma p}G_{\mu\nu}G_{\sigma\rho} \tag{2}$$

$s \notin S_2$: Negative transpose of $r \notin S_2$

## Elements added to diagonal of Hessian matrix $\frac{d^2\mathcal{J}}{d\kappa_{rs}{}^2}$

$r \in S_1$:

$$2\sum_{G}^{h}\sum_{(S_1,S_2)\in\mathcal{S}_G}\sum_{\bar{p}\notin S_2}\sum_{\mu\nu\sigma\rho} c^*_{\mu s}c^*_{\sigma s}c'_{\nu\bar{p}}c'_{\rho\bar{p}}G_{\mu\nu}G_{\sigma\rho} \tag{3}$$

$s \in S_1$: Transpose of $r \in S_1$

$r \notin S_2$:

$$2\sum_{G}^{h}\sum_{(S_1,S_2)\in\mathcal{S}_G}\sum_{p\in S_1}\sum_{\mu\nu\sigma\rho} c_{\nu s}c_{\rho s}c'^*_{\mu p}c'^*_{\sigma p}G_{\mu\nu}G_{\sigma\rho} \tag{4}$$

$s \notin S_2$: Transpose of $r \notin S_2$

$r \in S_1$ and $s \notin S_2$:

$$-2\sum_{G}^{h}\sum_{(S_1,S_2)\in\mathcal{S}_G}\sum_{\mu\nu\sigma\rho}\left(c'^*_{\mu r}c_{\nu r}c^*_{\sigma s}c'_{\rho s} + 2c'^*_{\mu r}c'_{\nu s}c^*_{\sigma s}c_{\rho r} + c^*_{\mu s}c'_{\nu s}c'^*_{\sigma r}c_{\rho r}\right)G_{\mu\nu}G_{\sigma\rho} \tag{5}$$

$r \notin S_2$ and $s \in S_1$: Transpose of $r \in S_1$ and $s \notin S_2$

## Elements added to Hessian matrix multiplied by trial function $(\mathbf{Hx})_{rs}$

$r \in S_1$:

$$4\sum_{G}^{h}\sum_{\mu\nu\sigma\rho}\sum_{u}\left(\sum_{t\in S_1}\sum_{(S_1,S_2)\in\mathcal{S}_G}\sum_{\bar{p}\notin S_2}\delta_{rt}c^*_{\mu u}c'_{\nu\bar{p}}c^*_{\sigma s}c'_{\rho\bar{p}} + \sum_{t\notin S_2}c^*_{\sigma s}c'^*_{\mu r}\left(c'_{\rho t}c_{\nu u} + c_{\rho u}c'_{\nu t}\right)\right)G_{\mu\nu}G_{\sigma\rho}x_{tu} \tag{6}$$

$s \in S_1$: Negative transpose of $r \in S_1$

$r \notin S_2$:

$$4\sum_{G}^{h}\sum_{\mu\nu\sigma\rho}\sum_{u}\left(\sum_{t\in S_1}c'_{\nu r}c_{\rho s}\left(c^*_{\mu u}c'^*_{\sigma t} + c'^*_{\mu t}c^*_{\sigma u}\right) + \sum_{t\notin S_2}\sum_{(S_1,S_2)\in\mathcal{S}_G}\sum_{p\in S_1}\delta_{rt}c'^*_{\mu p}c_{\nu u}c'^*_{\sigma p}c_{\rho s}\right)G_{\mu\nu}G_{\sigma\rho}x_{tu} \tag{7}$$

$s \notin S_2$: Negative transpose of $r \notin S_2$

# Symmetry-invariant blocks

## Pipek-Mezey occupied orbitals

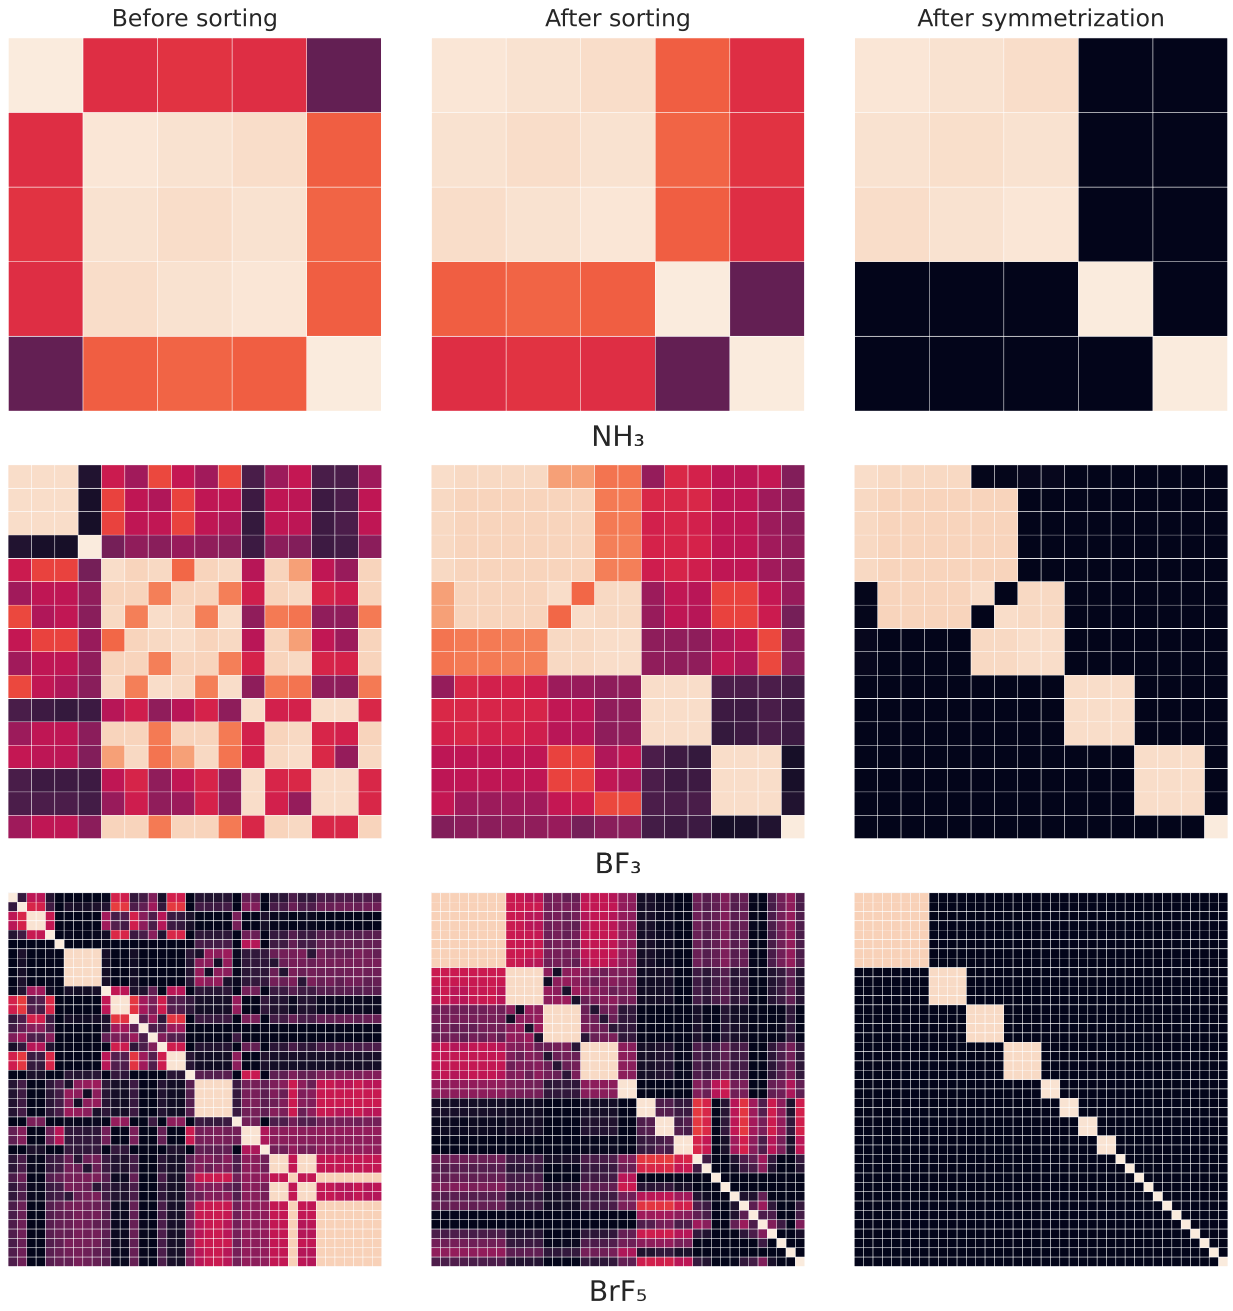


Figure S1: Heatmaps of $\boldsymbol{G}^{\Sigma}$ for Pipek-Mezey localized occupied orbitals of $NH_3$, $BF_3$, and $BrF_5$ before symmetrization, after sorting by the reverse Cuthill-McKee algorithm, and after symmetrization. Orbital indices are plotted along both the x-/y-axes and the employed color map is logarithmic, ranging in values of $\boldsymbol{G}^{\Sigma}$ from $10^{-13}$ (black) to 1 (bright beige tone).

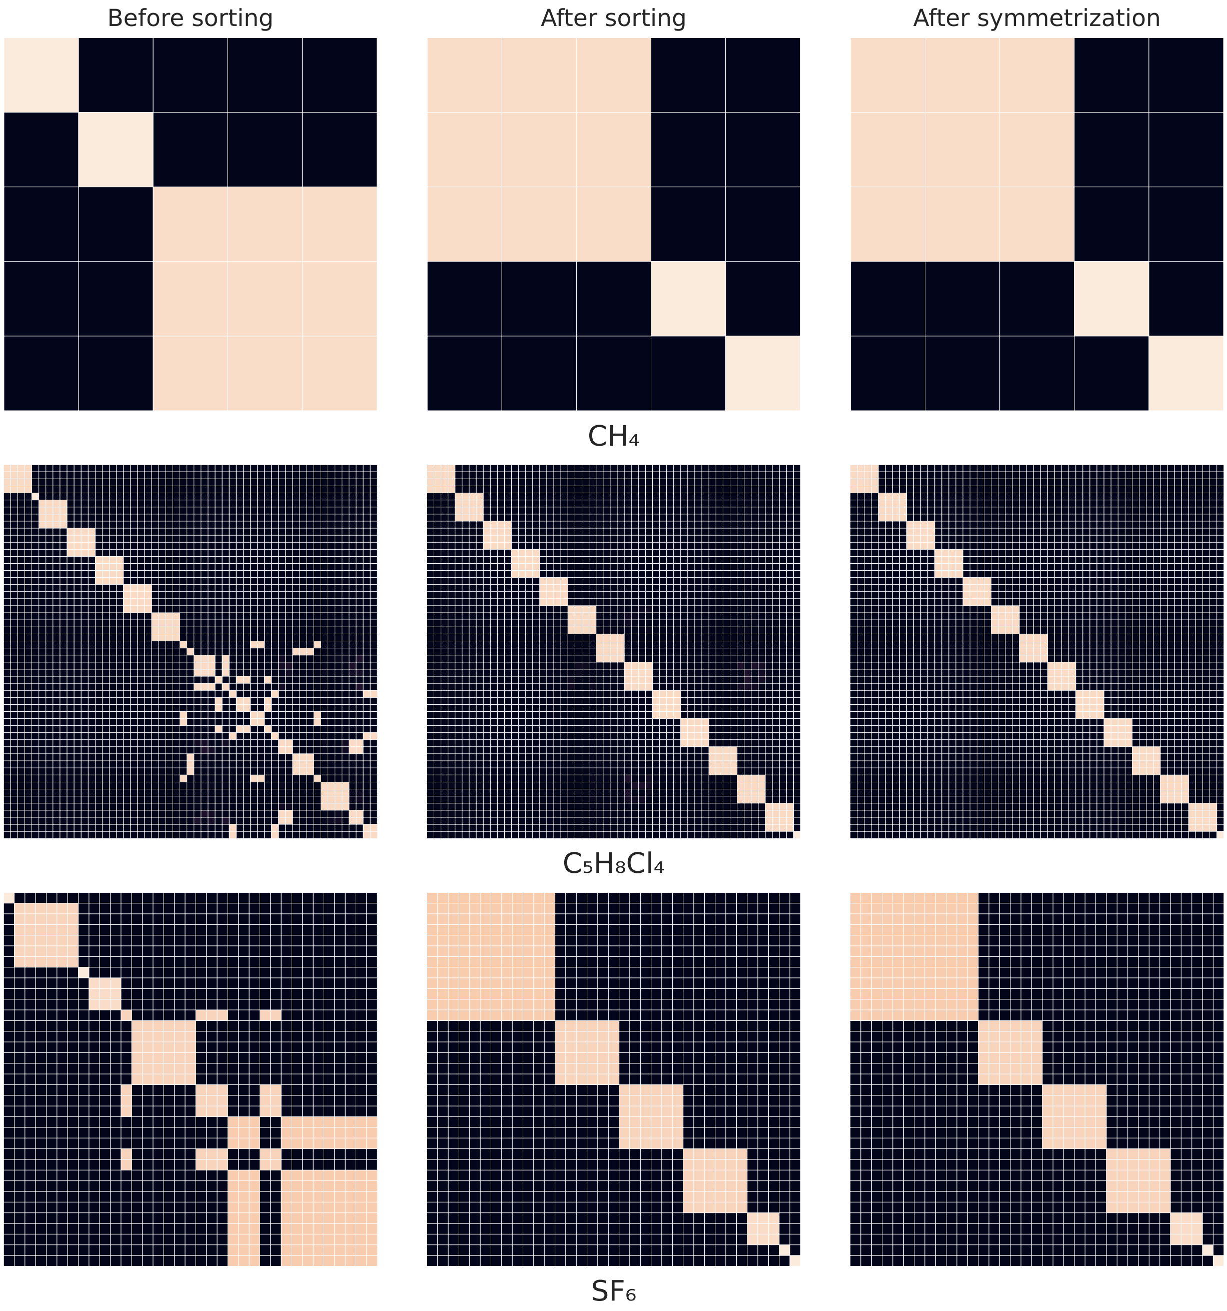


Figure S2: Same plot as Fig. S1, but for occupied orbitals of $CH_4$, $C_5H_8Cl_4$, and $SF_6$.

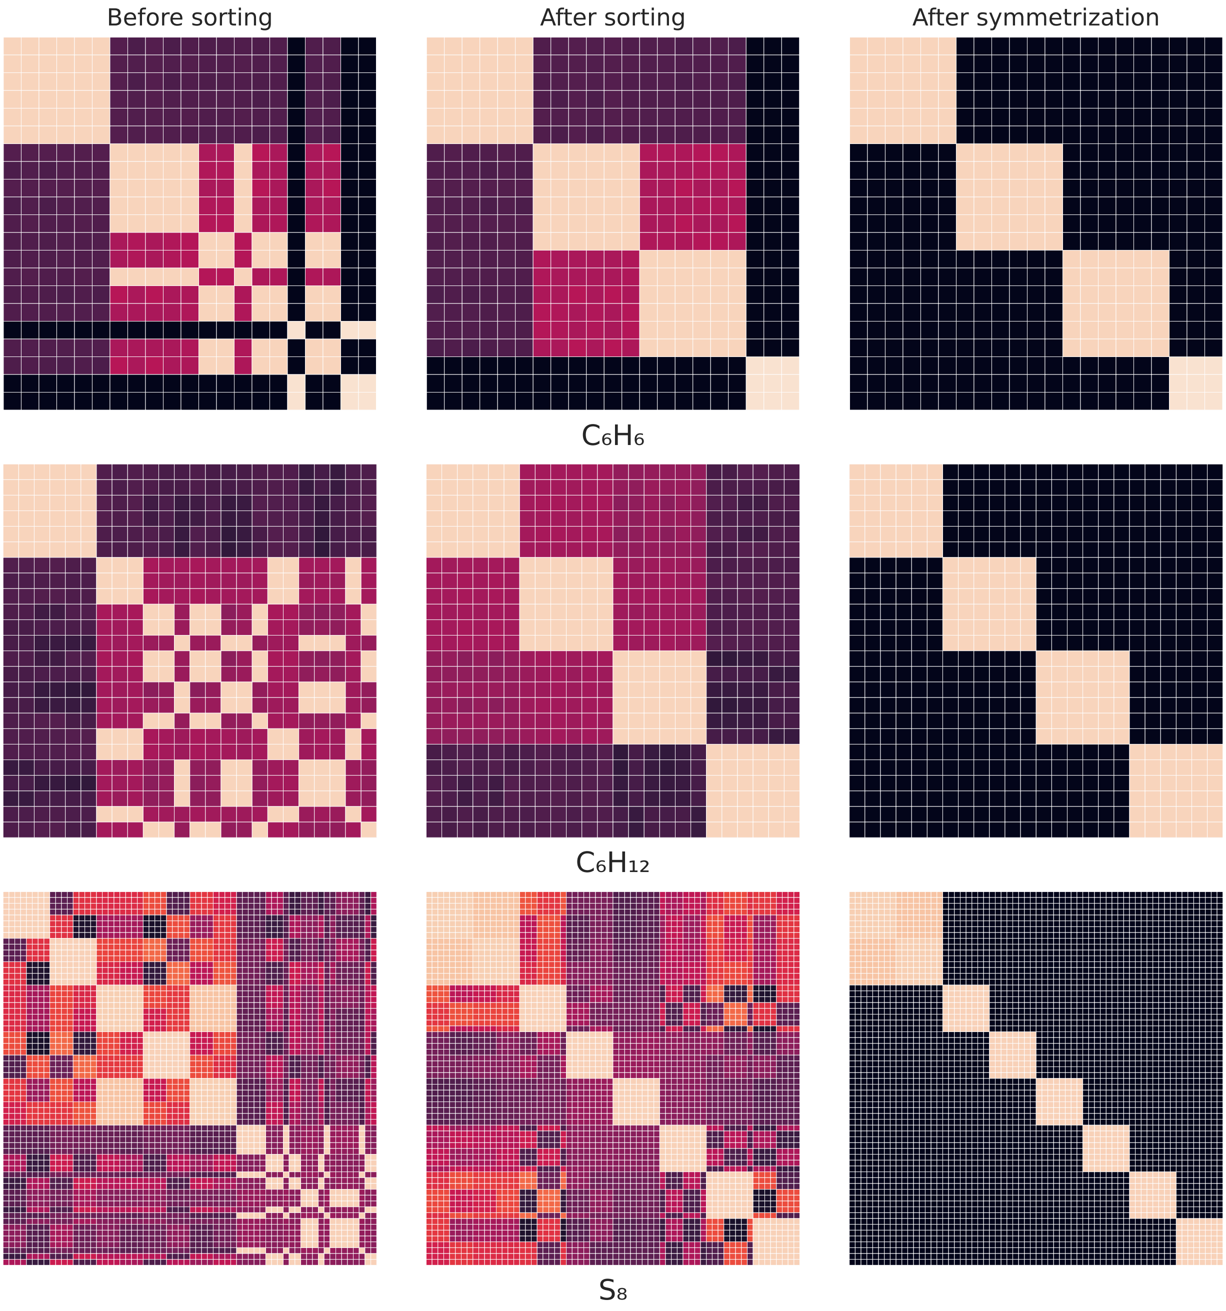


Figure S3: Same plot as Fig. S1, but for occupied orbitals of $C_6H_6$, $C_6H_{12}$, and $S_8$.

## Pipek-Mezey virtual orbitals

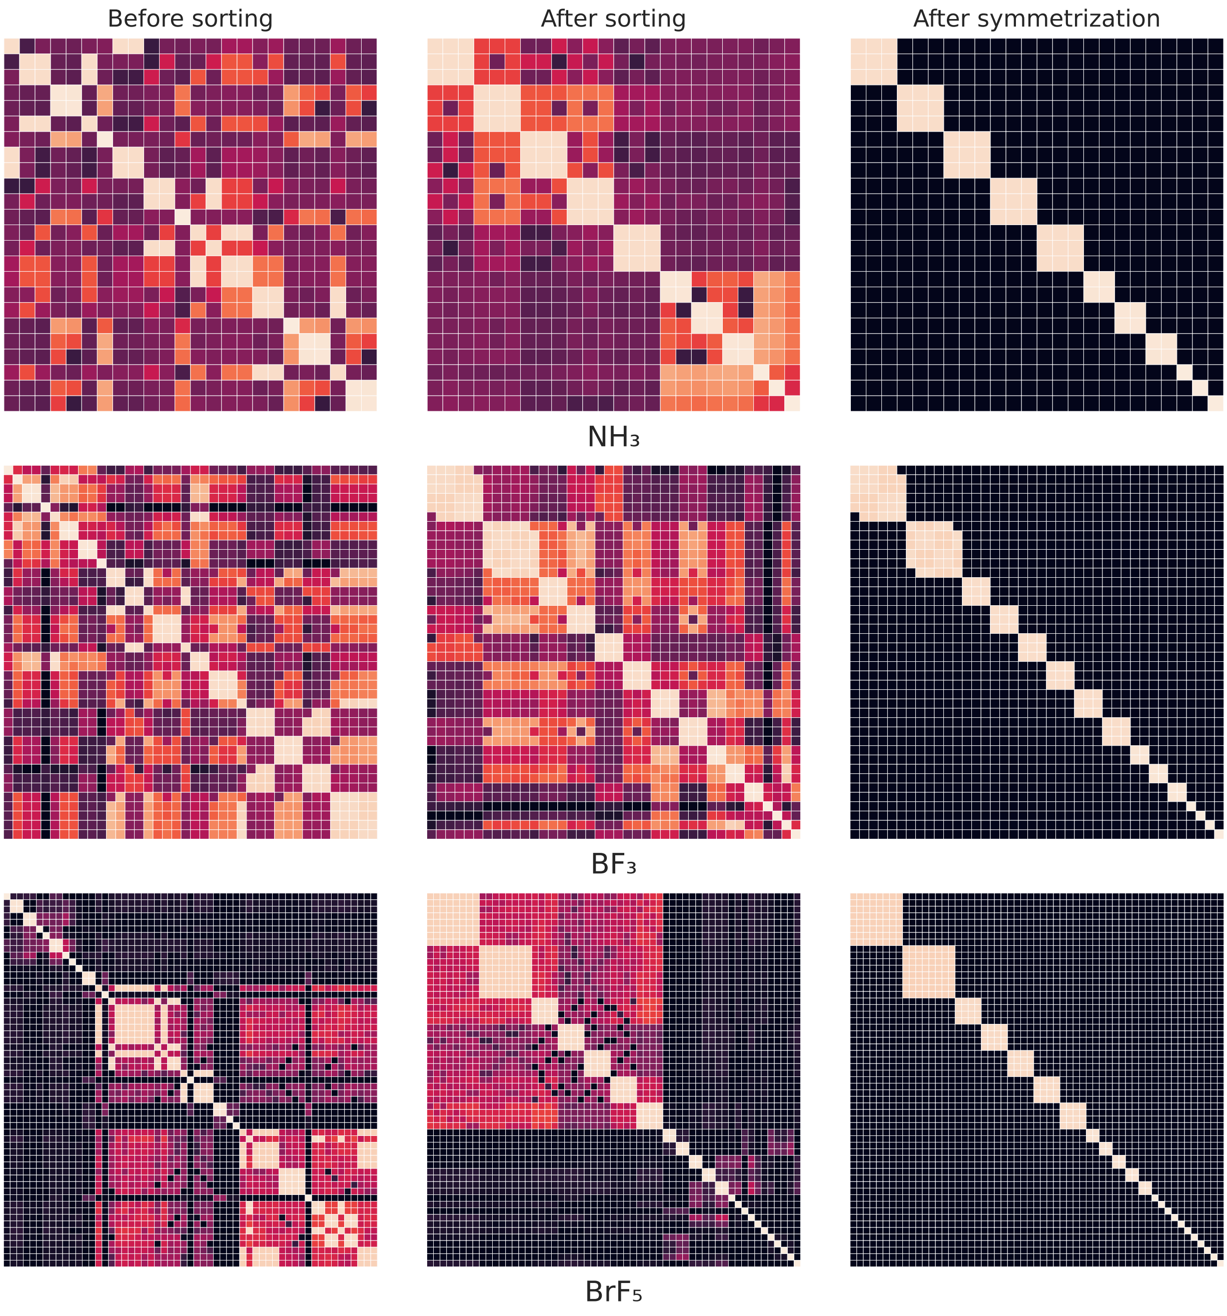


Figure S4: Same plot as Fig. S1, but for the virtual orbitals of these molecules instead.

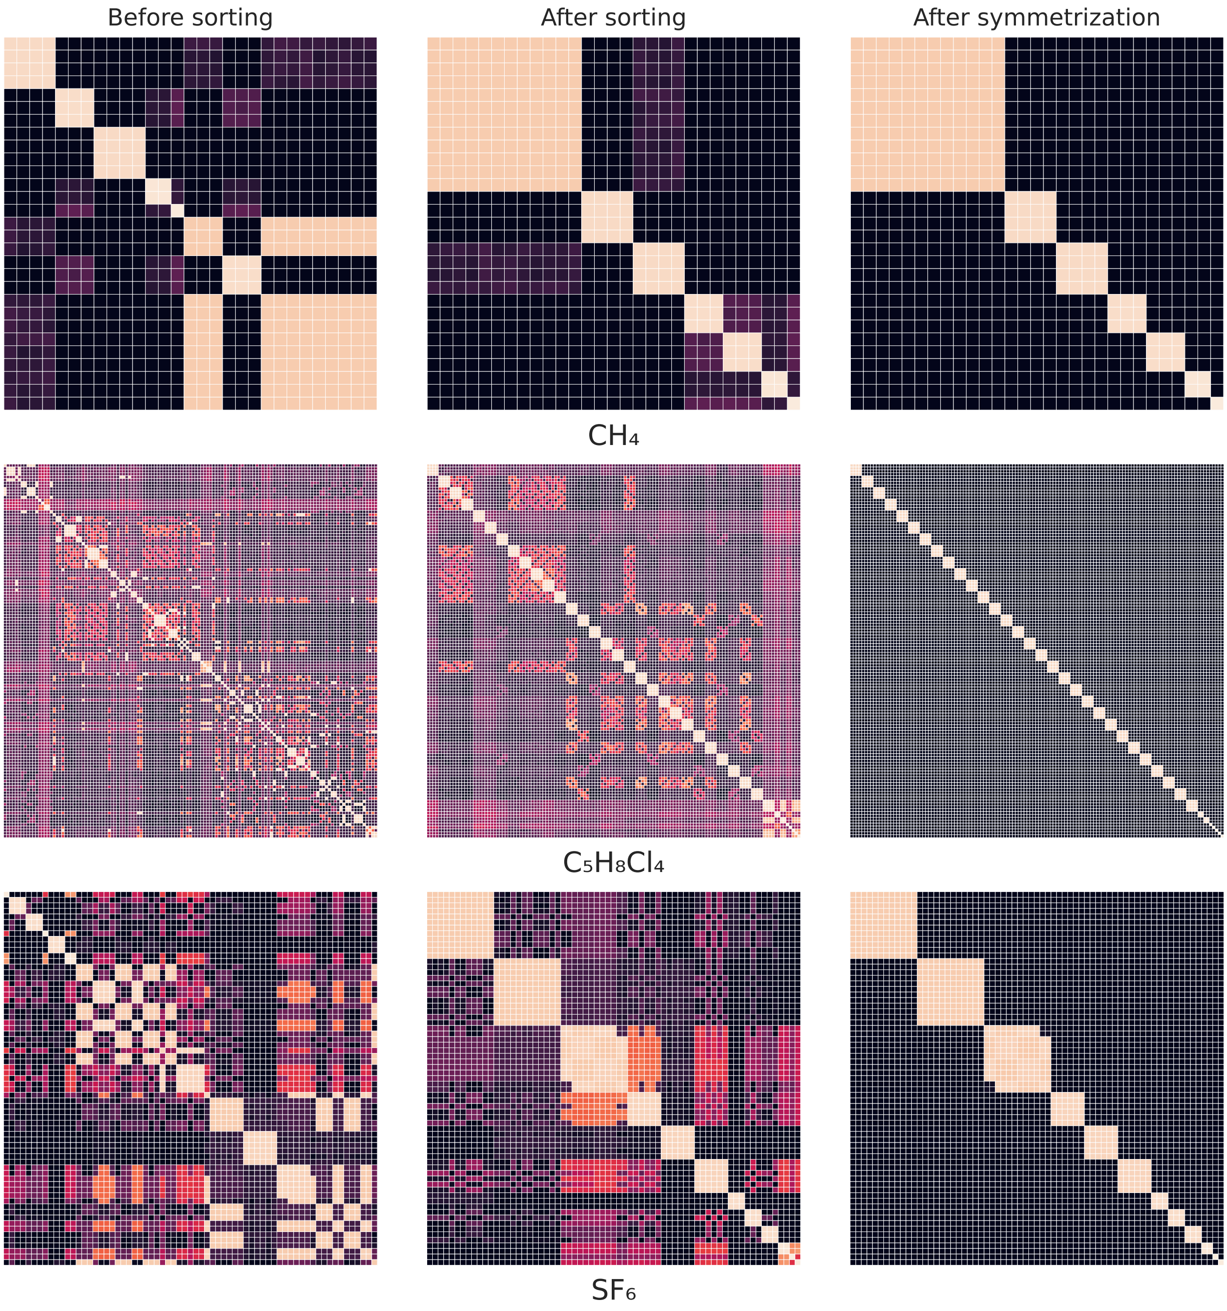


Figure S5: Same plot as Fig. S2, but for the virtual orbitals instead.

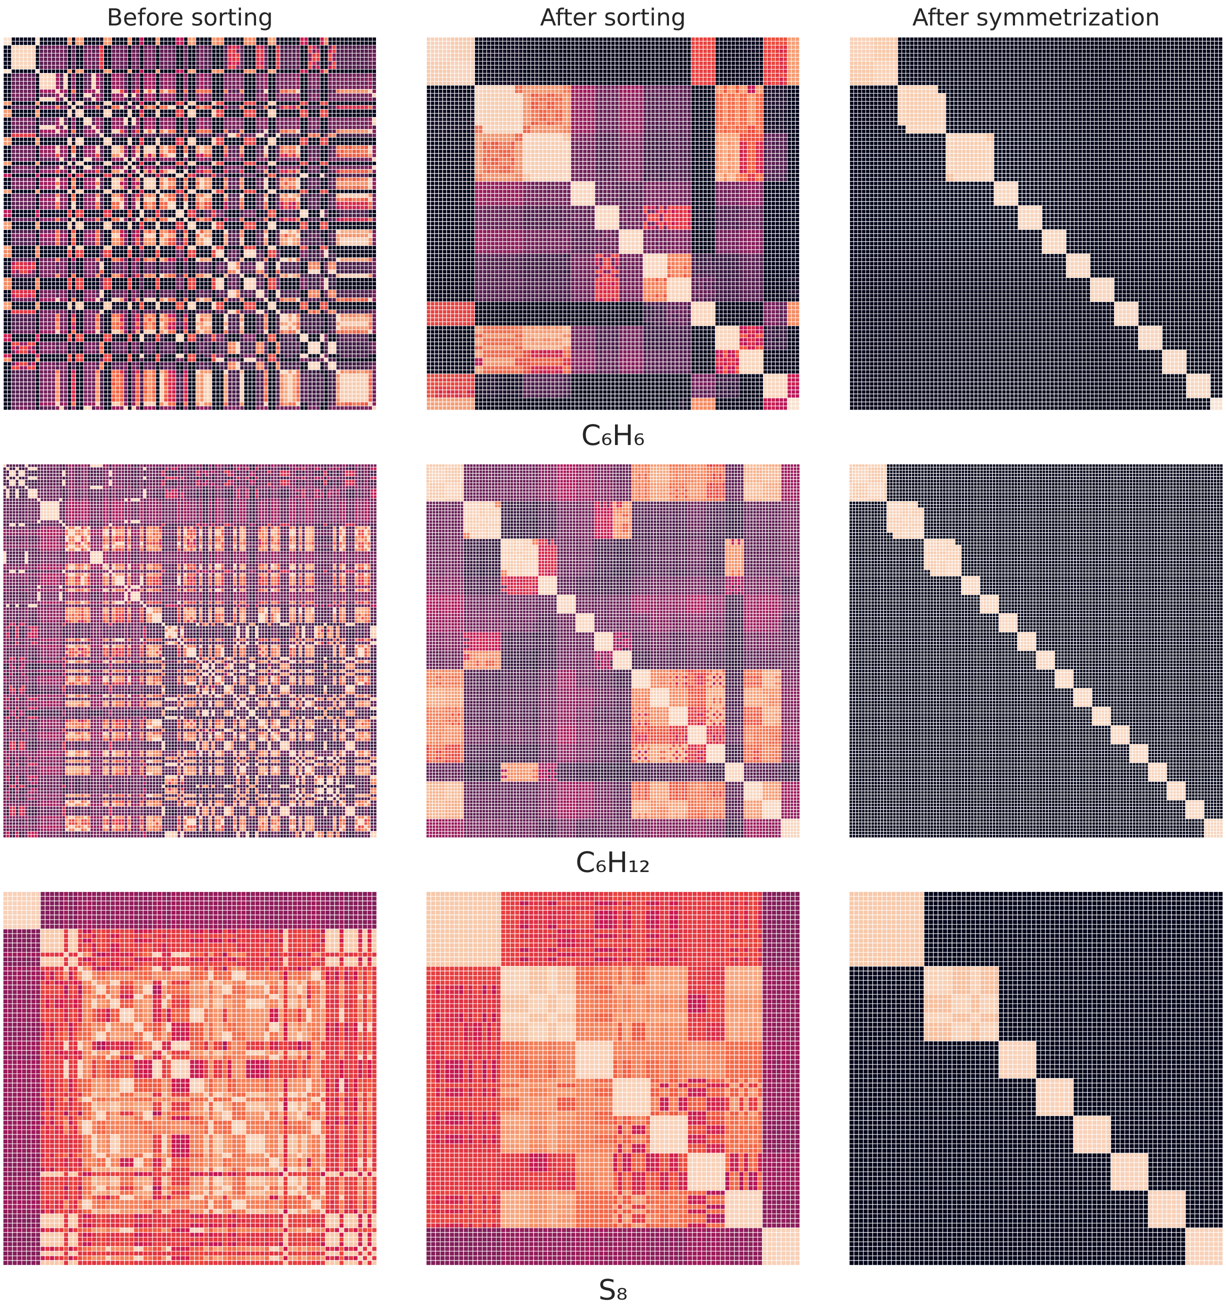


Figure S6: Same plot as Fig. S3, but for the virtual orbitals instead.

## Foster-Boys occupied orbitals

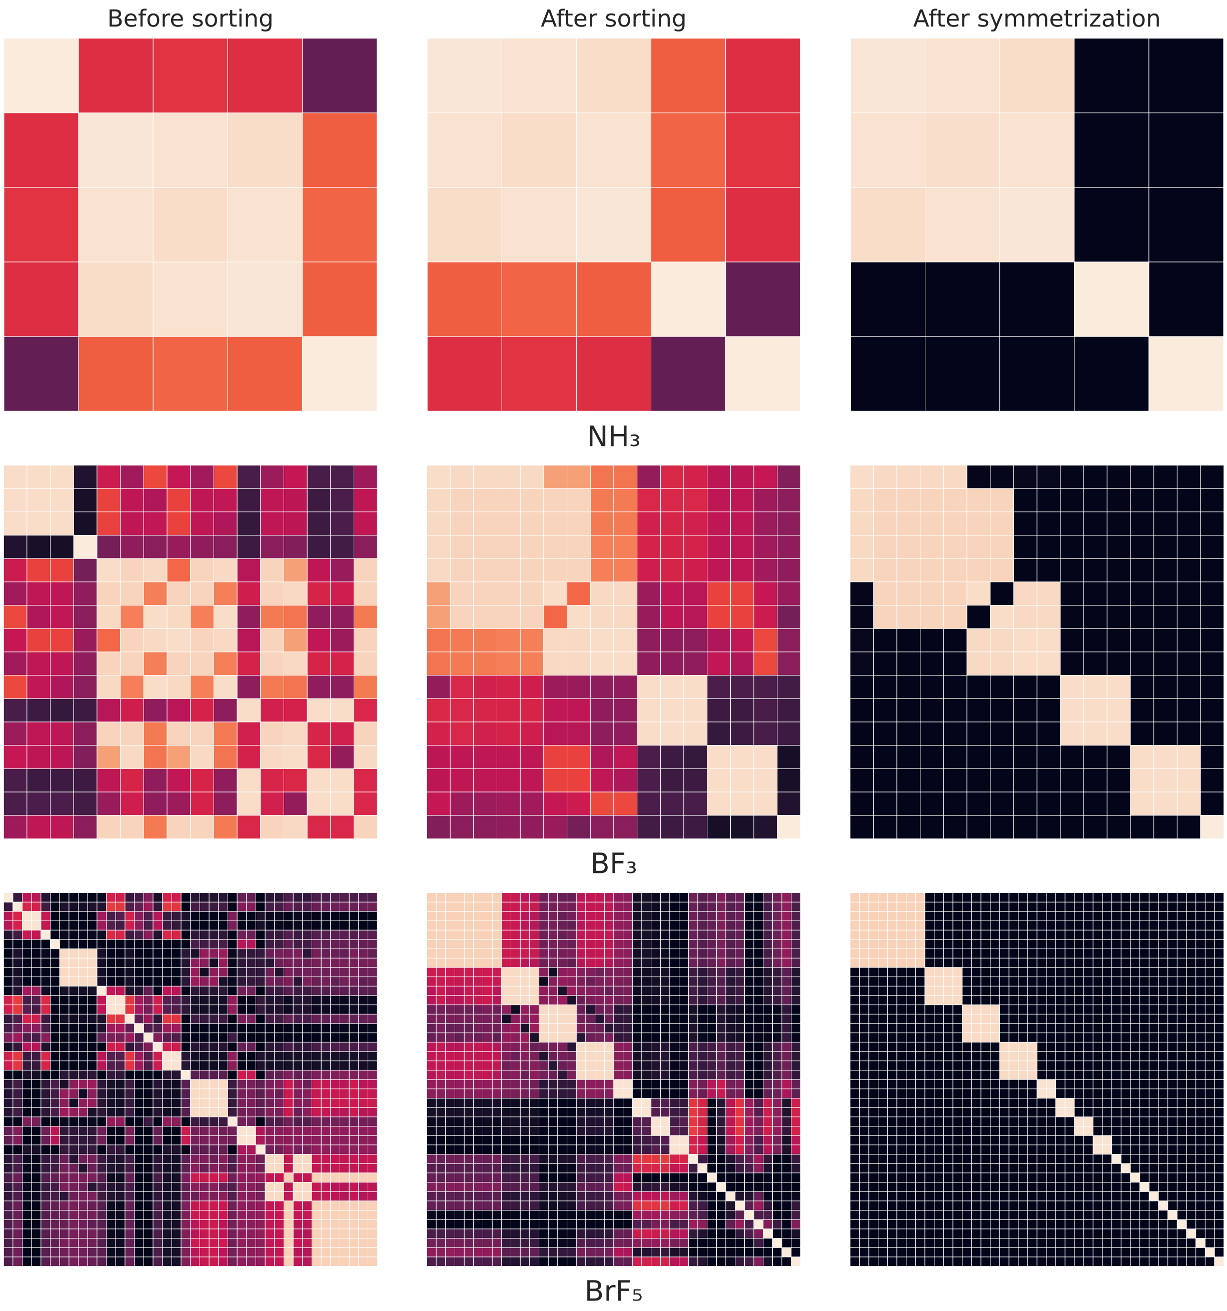


Figure S7: Same plot as Fig. S1, but for Foster-Boys localized orbitals instead.

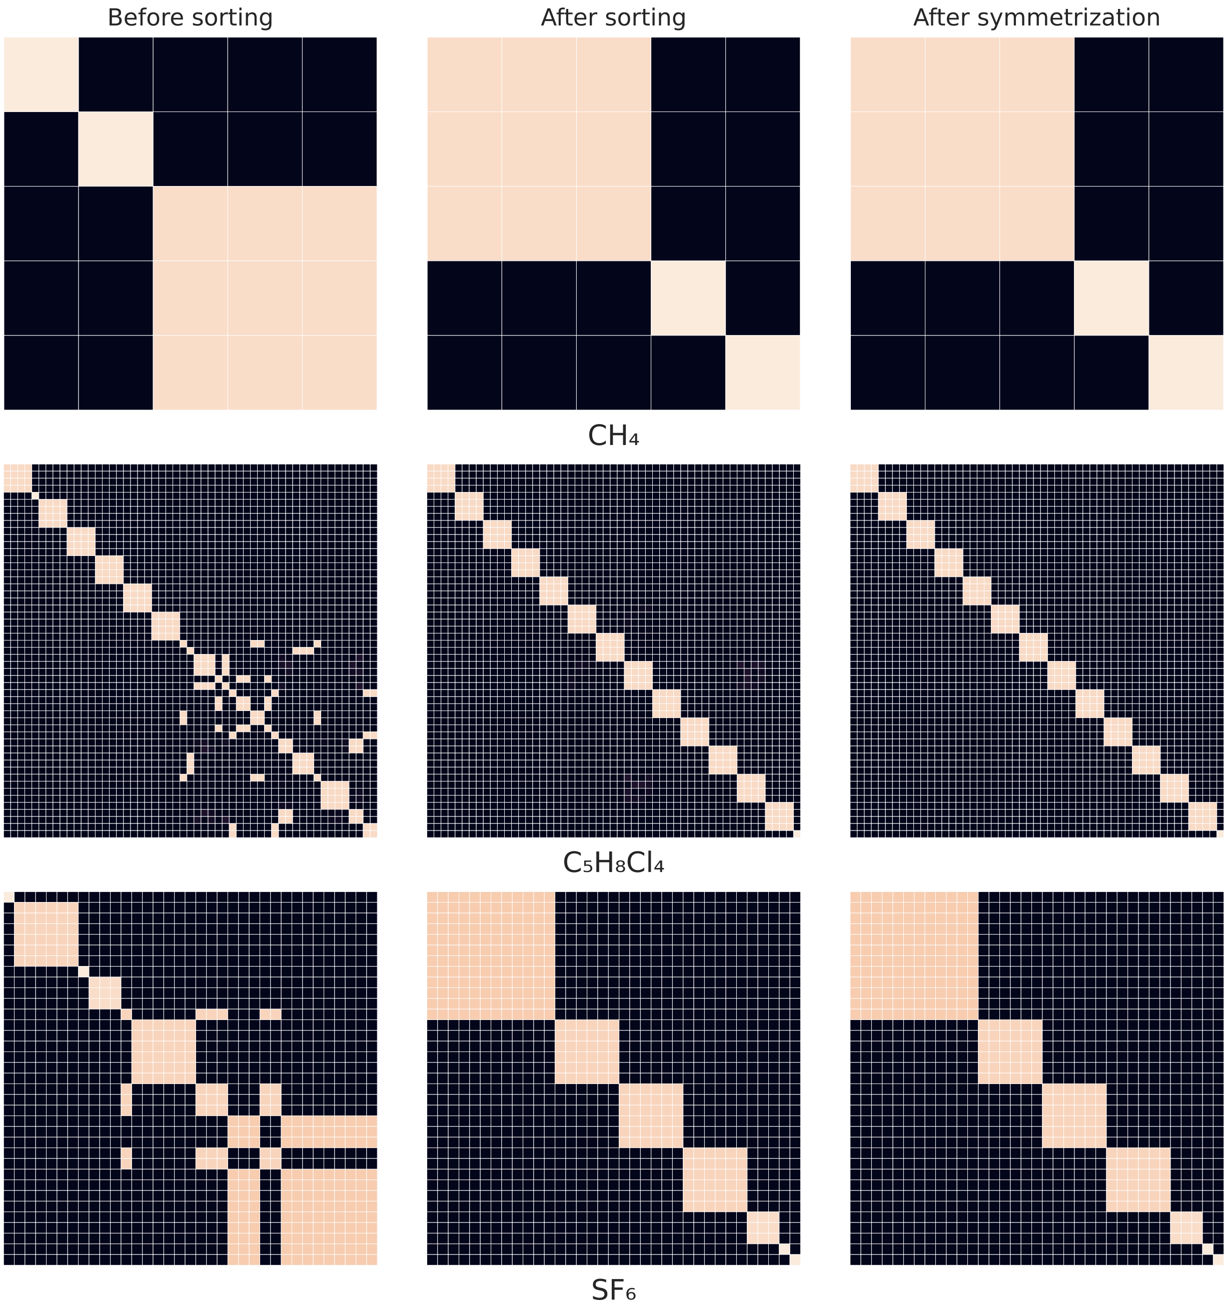


Figure S8: Same plot as Fig. S2, but for Foster-Boys localized orbitals instead.

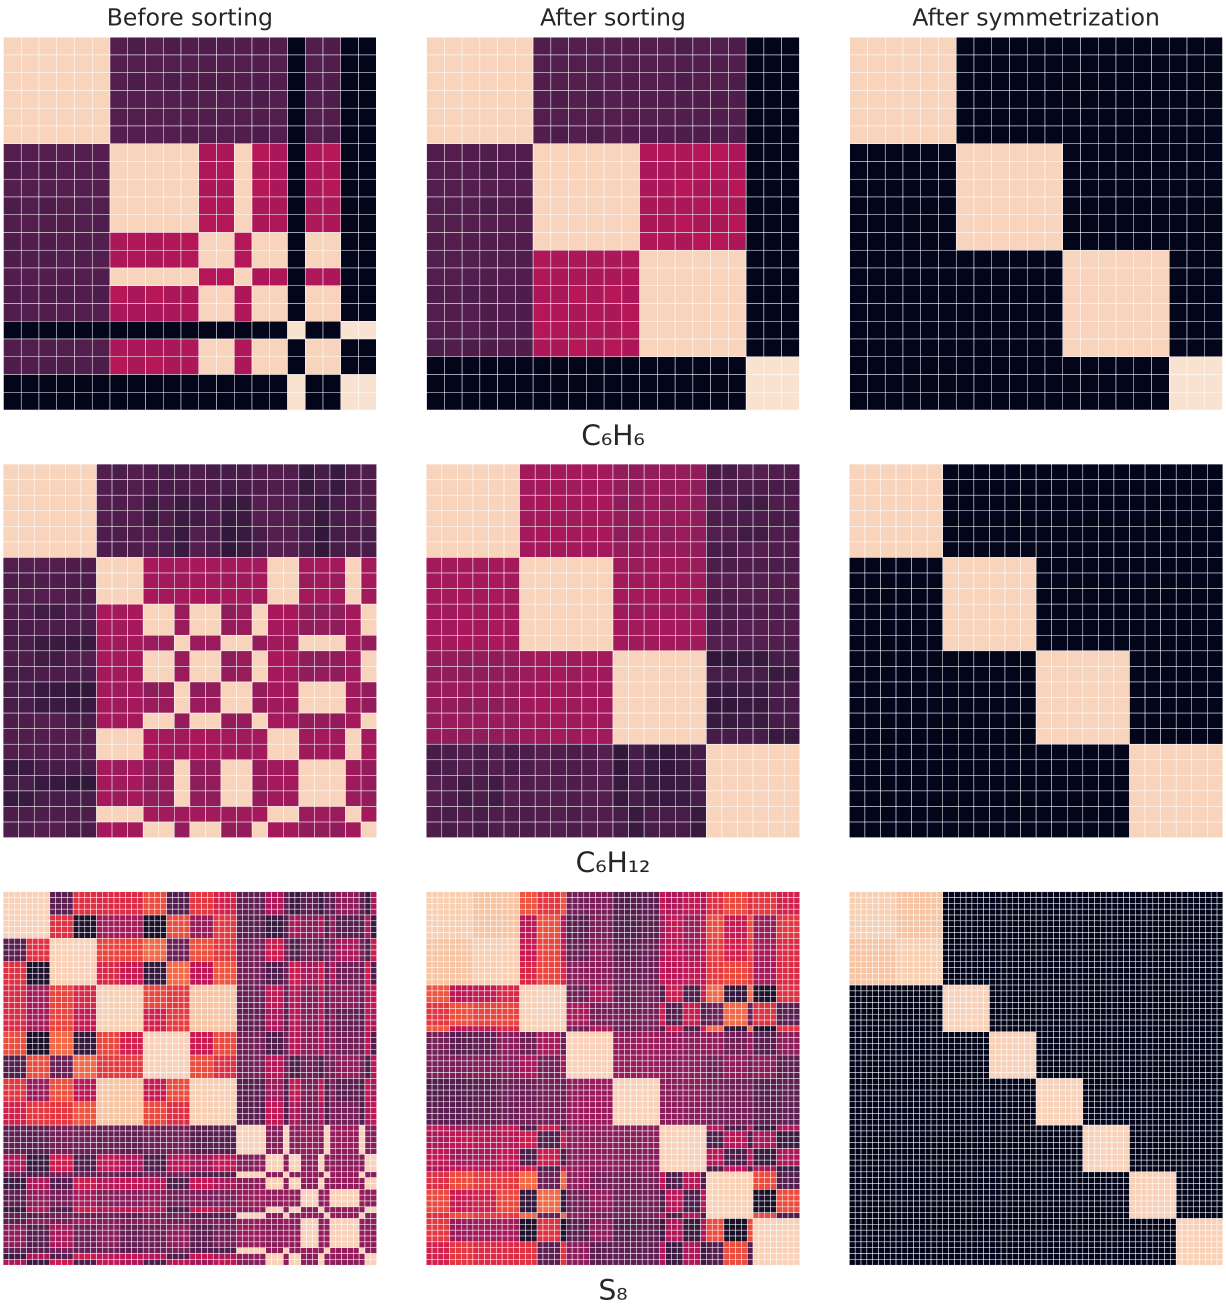


Figure S9: Same plot as Fig. S3, but for Foster-Boys localized orbitals instead.

## Foster-Boys virtual orbitals

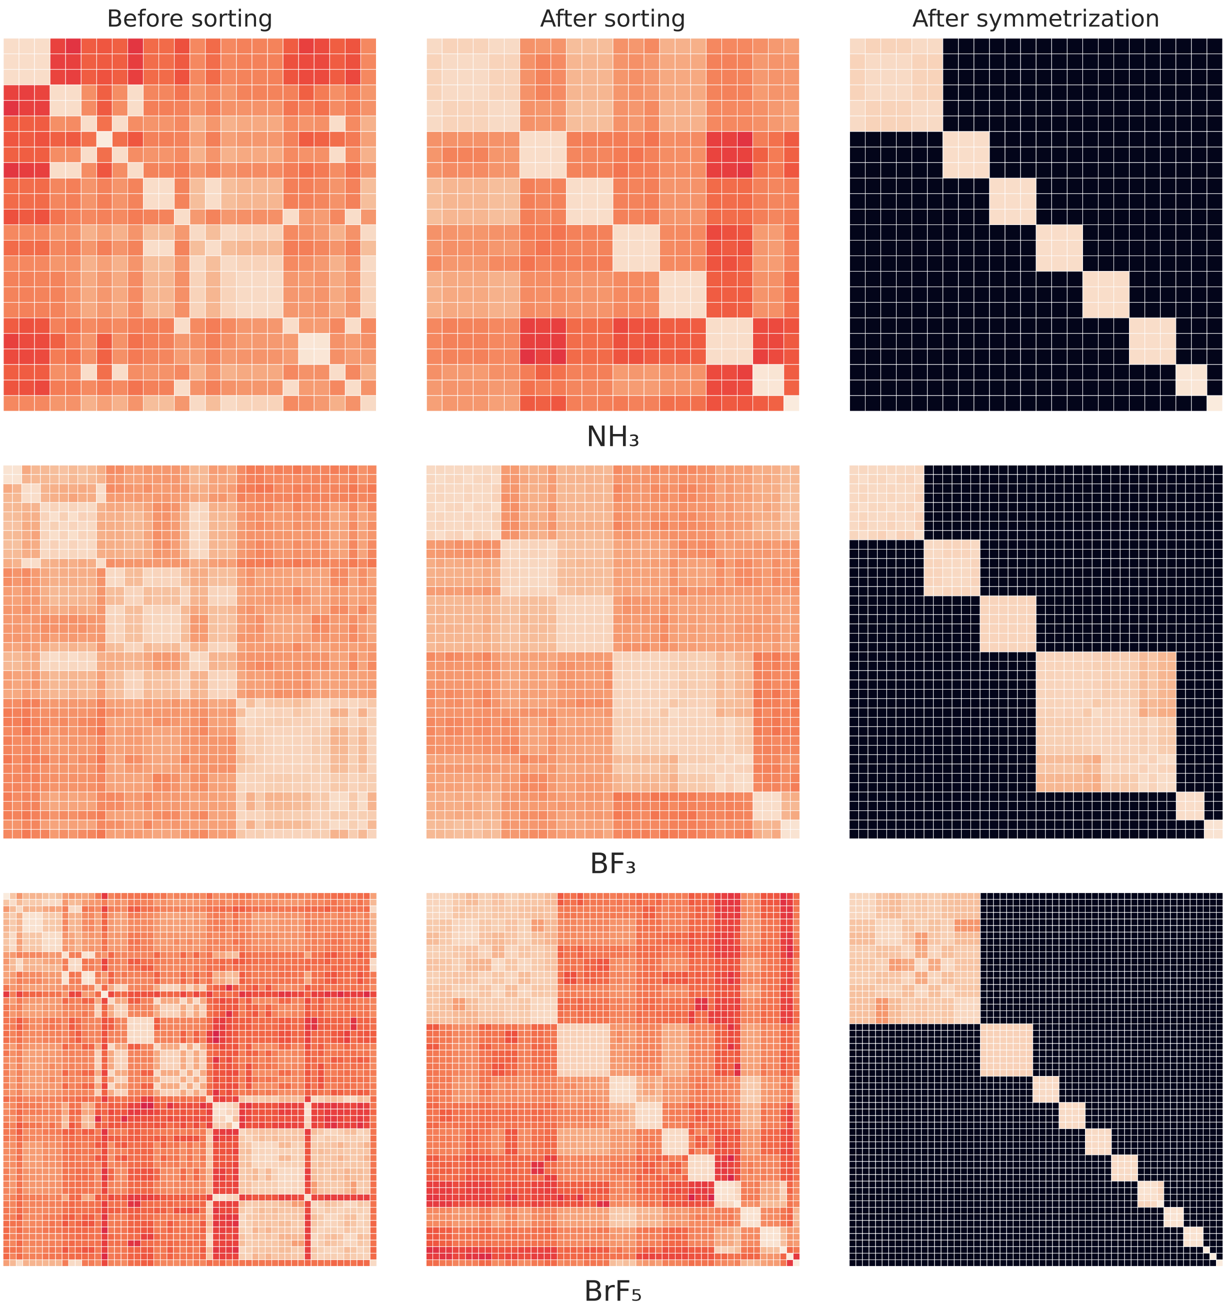


Figure S10: Same plot as Fig. S4, but for Foster-Boys localized orbitals instead.

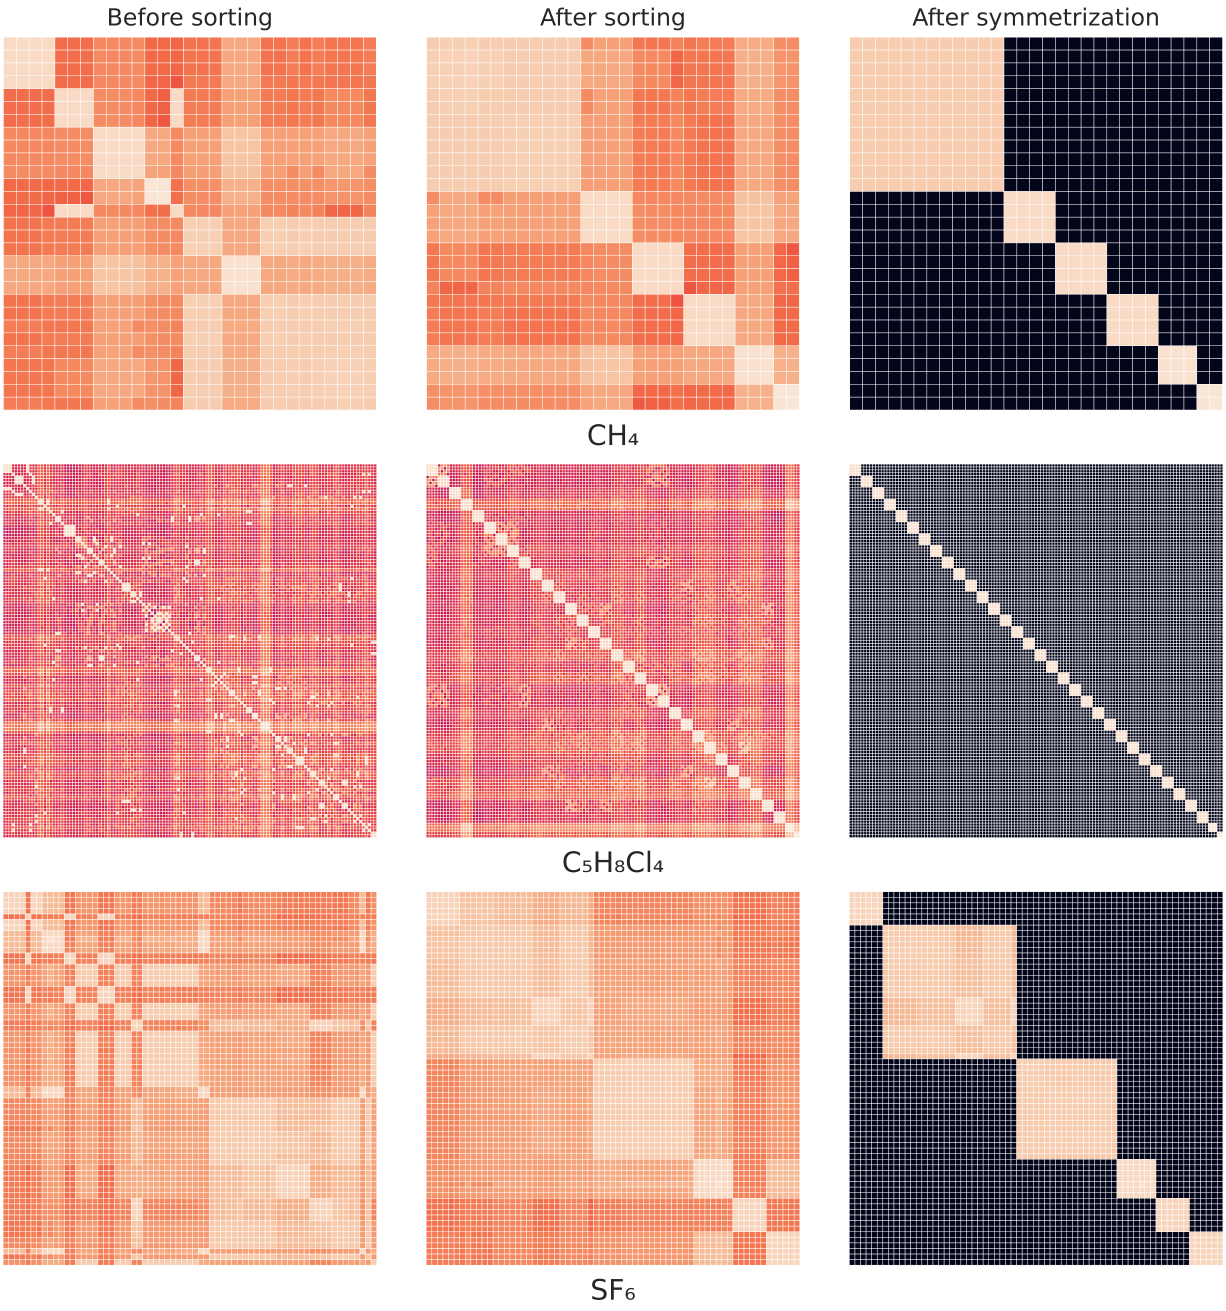


Figure S11: Same plot as Fig. S5, but for Foster-Boys localized orbitals instead.

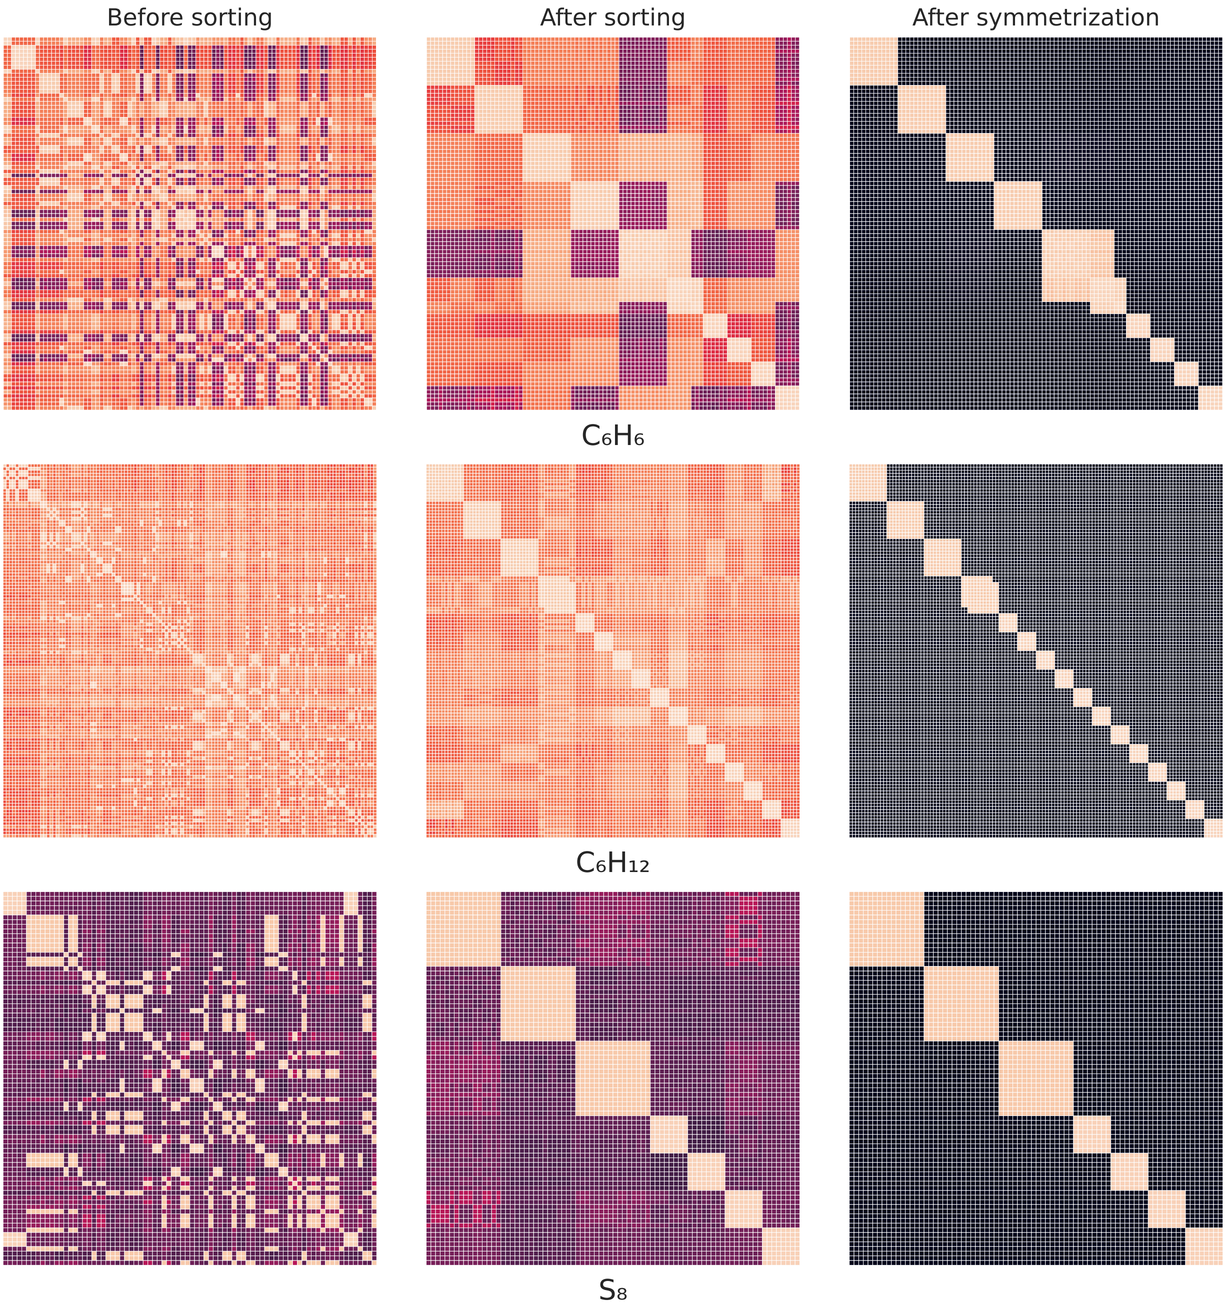


Figure S12: Same plot as Fig. S6, but for Foster-Boys localized orbitals instead.

## Second moment orbital spread

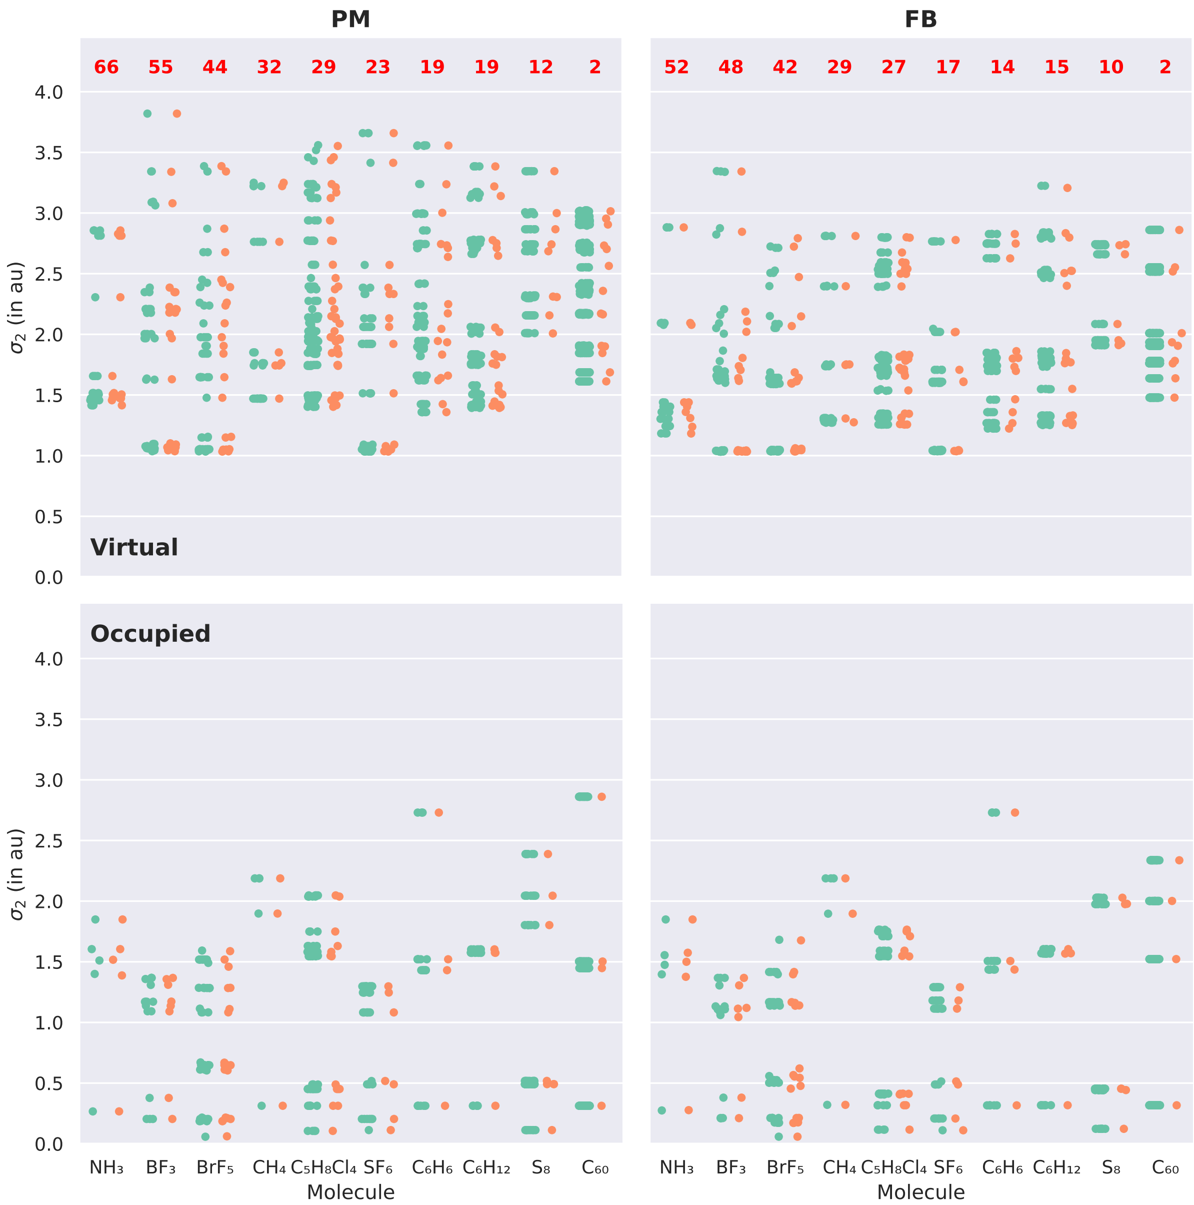


Figure S13: Second-moment orbital spreads ($\sigma_2^p$) of PM and FB localized orbitals. Results for orbitals before and after the symmetrization are displayed in green and orange, respectively, and the percentage of symmetry-unique orbitals for every molecule is displayed in red.
